# Supplementary material for: Approximate Caching for Efficiently Serving Diffusion Models
Source: arXiv:2312.04429 source file (2023-12-07)
Supplement: Supplementary file 1 [file appendix.tex]

\appendix

\section{Concept Development in Image Generation} \label{sec:motivation_example}

This section gives a motivating example on how various concepts/characteristics develop during image generation ~\cite{zhang2023prospect}.

\begin{figure}[h!]
\centering
  \includegraphics[width=1.0\columnwidth]{figures/placeholders/Screenshot 2023-09-10 at 3.49.00 PM.png}
  \caption{Generation across K}
  \label{fig:motivation_example}
\end{figure}

In Figure \ref{fig:motivation_example}, we present an illustrative example of image generation using a prompt that encompasses various aspects, including color, layout, content, size, style, and more. We divide the generation steps into four distinct time buckets, labeled as t1, t2, t3, and t4, with each bucket having a unique role in shaping different facets of the image. The formation of color initiates in t1 and becomes relatively stable by t2. Style, here referring to generating a digital art image in the style of a detailed photograph, commences in t1 and experiences significant development in t2. The image's content, featuring a bird and leaves, begins to manifest partially towards the end of t2, with substantial development occurring in t3. Layout, which dictates the positioning of elements like the blackbird, starts its formation in t1 and progresses towards the end of this phase. By the time we reach t4, most aspects of the image are firmly established, with this final bucket primarily responsible for fine-tuning and enhancing details and clarity.
